# Supplementary material for: KeepAugment: A Simple Information-Preserving Data Augmentation Approach
Source: arXiv:2011.11778 source file (2020-11-23)
Supplement: Supplementary file 1 [file appendix.tex]

\appendix

\section{Additional Empirical Study}

In Figure~\ref{fig:ndr_cutout_randaug}, 
we further exam the fidelity of the augmented data 
using an independent trained model $f^*$, which is EfficientNet-B5 pretrained on ImageNet and finetuned on CIFAR-10 with 99\% CIFAR-10 validation accuracy.
We define the fidelity of an data augmentation $\mathcal A$ to be
$$ 
\mathcal F(\mathcal A) = \E_{x\sim \mathcal D}[\ind(f^*(x)=f^*(\mathcal A(x)))],
$$
which is the probability that the transformed data has the same label as the original data under the oracle model. 
As shown in Figure~\ref{fig:ndr_cutout_randaug}, the fidelity decreases monotonically w.r.t. both cutout length and distortion magnitude in RandAugment, 
which clearly indicates the presence of misinformation when data augmentation is applied too aggressively. 

\begin{figure}[h]
  \begin{center}
  \raisebox{3em}{\rotatebox{90}{Fidelity}}
   \includegraphics[width=0.45\textwidth]{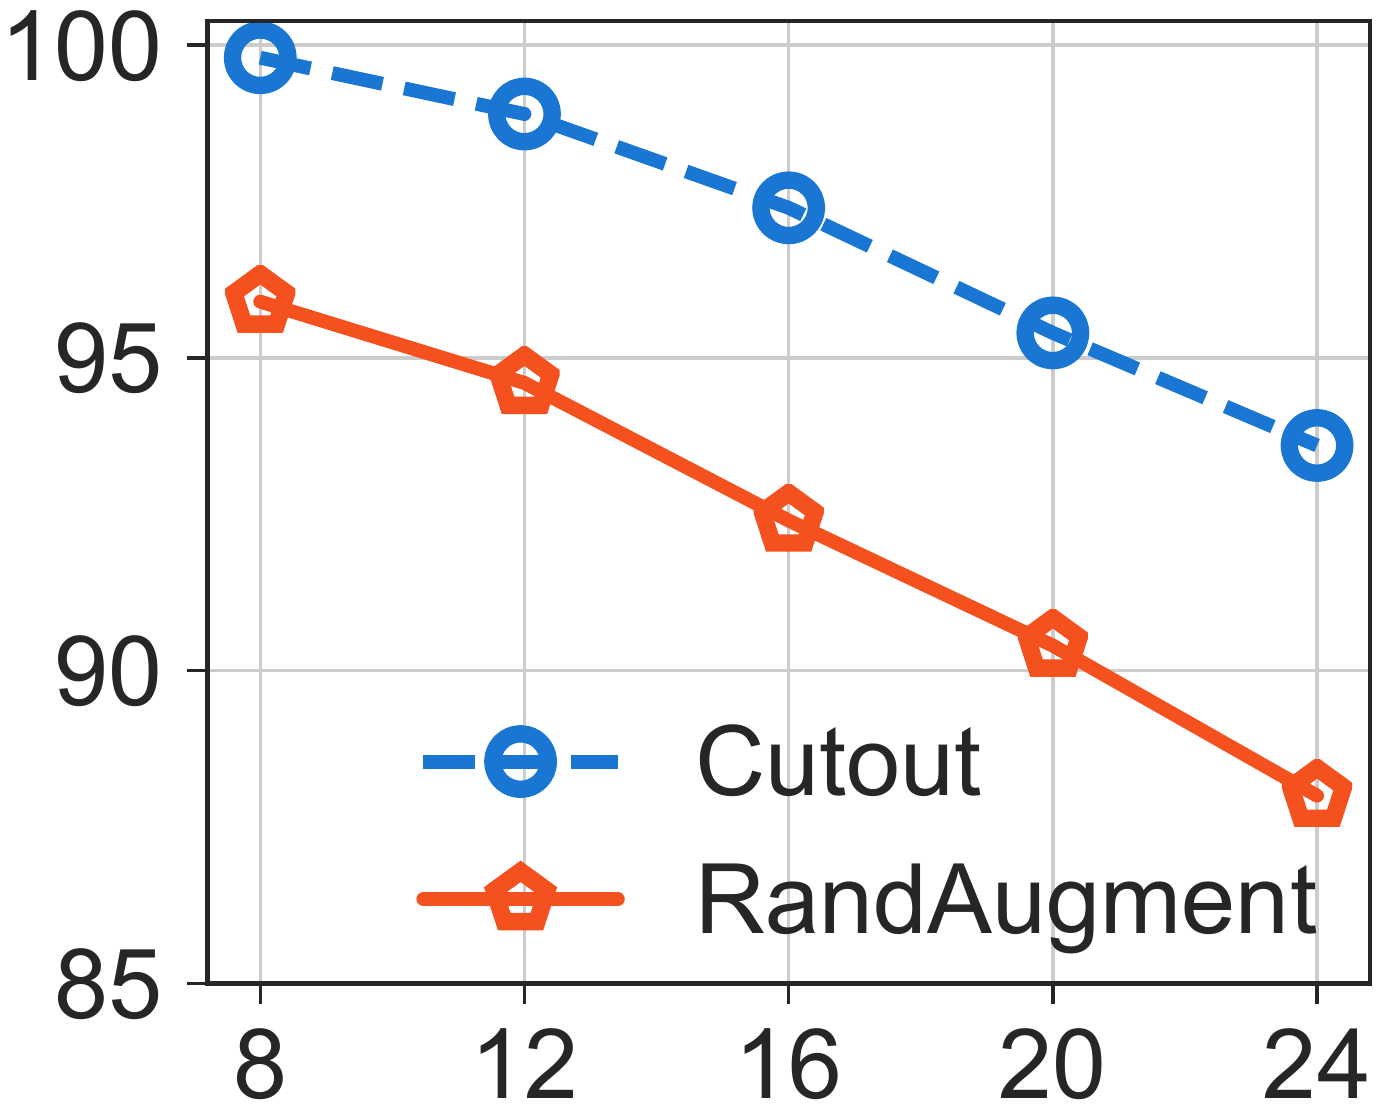} \\
  \end{center}
  \caption{Analysis of the information induced by data augmentation. The x-axis represents Cutout length (for \cutout) and Distortion magnitude (for \randaug). }
\label{fig:ndr_cutout_randaug}
\end{figure}
